# Supplementary material for: The Medium Amplitude Response of Nonlinear Maxwell-Oldroyd Type Models in Simple Shear
Source: arXiv:2103.02560 ancillary file (2021-03-03)
Supplement: Supplementary file 1 [file Maxwell-Oldroyd_SI.pdf]

Supporting Information:

# The Medium Amplitude Response of Nonlinear Maxwell-Oldroyd Type Models in Simple Shear

Kyle R. Lennon[1], Gareth H. McKinley[2], and James W. Swan[1]

[1] *Department of Chemical Engineering, Massachusetts Institute of Technology, Cambridge, MA 02142*

[2] *Department of Mechanical Engineering, Massachusetts Institute of Technology, Cambridge, MA 02139*

## S1 Derivation of the MAPS Response of the Generalized Nonlinear Maxwell Model

In simple shear flow, we can write $\mathbf{u} = \gamma_0 s(t) x_e \mathbf{e}_1$ for some time-dependent protocol $s(t)$. The components of the non-Newtonian extra stress tensor in this case may be written as a power series in $\gamma_0$:

$$\boldsymbol{\sigma} = \gamma_0 \boldsymbol{\sigma}^{(1)} + \gamma_0^2 \boldsymbol{\sigma}^{(2)} + \gamma_0^3 \boldsymbol{\sigma}^{(3)} + O(\gamma_0^4). \tag{S1}$$

Substituting the flow field and the power series for the stress into the cubic Maxwell model, and retaining only terms that are linear in $\gamma_0$, gives:

$$\sigma_{12}^{(1)} + \lambda_1 \frac{d\sigma_{12}^{(1)}}{dt} = \eta_0 \left( s(t) + \lambda_2 \frac{ds(t)}{dt} \right), \tag{S2}$$

and that no other component (besides the symmetric element $\sigma_{21}^{(1)}$) is nonzero at first order in $\gamma_0$. Taking the Fourier transform gives:

$$\hat{\sigma}_{12}^{(1)}(\omega) = \eta_0 \left( \frac{1 + i\lambda_2\omega}{1 + i\lambda_1\omega} \right) \hat{s}(\omega), \tag{S3}$$

and the resulting expression for the linear complex viscosity:

$$\eta_1^*(\omega) = \eta_0 \left( \frac{1 + i\lambda_2\omega}{1 + i\lambda_1\omega} \right). \tag{S4}$$

## S1.1 Leading Order Normal Stresses

At second order, we find that the shear stress component $\sigma_{12}^{(2)} = 0$ for all time, and the normal stresses are governed by:

$$\sigma_{11}^{(2)} + \lambda_1 \frac{d\sigma_{11}^{(2)}}{dt} - (\lambda_1 + \mu_1 - \nu_1) s(t) \sigma_{12}^{(1)} + \frac{\alpha_1}{\eta_0} (\sigma_{12}^{(1)})^2 - \frac{\beta_1}{\eta_0} (\sigma_{12}^{(1)})^2 + \zeta(\sigma_{11}^{(2)} + \sigma_{22}^{(2)} + \sigma_{33}^{(2)}) = \eta_0(-\lambda_2 - \mu_2 + \nu_2) s(t)^2, \tag{S5a}$$

$$\sigma_{22}^{(2)} + \lambda_1 \frac{d\sigma_{22}^{(2)}}{dt} - (-\lambda_1 + \mu_1 - \nu_1) s(t) \sigma_{12}^{(1)} + \frac{\alpha_1}{\eta_0} (\sigma_{12}^{(1)})^2 - \frac{\beta_1}{\eta_0} (\sigma_{12}^{(1)})^2 + \zeta(\sigma_{11}^{(2)} + \sigma_{22}^{(2)} + \sigma_{33}^{(2)}) = \eta_0(\lambda_2 - \mu_2 + \nu_2) s(t)^2, \tag{S5b}$$

$$\sigma_{33}^{(2)} + \lambda_1 \frac{d\sigma_{33}^{(2)}}{dt} + \nu_1 s(t) \sigma_{12}^{(1)} - \frac{\beta_1}{\eta_0} (\sigma_{12}^{(1)})^2 + \zeta(\sigma_{11}^{(2)} + \sigma_{22}^{(2)} + \sigma_{33}^{(2)}) = \eta_0 \nu_2 s(t)^2. \tag{S5c}$$

These equations may be combined to give expressions for the first and second normal stress differences at leading order ($N_1 = \sigma_{11} - \sigma_{22}$ and $N_2 = \sigma_{22} - \sigma_{33}$):

$$N_1^{(2)} + \lambda_1 \frac{dN_1^{(2)}}{dt} - 2\lambda_1 s(t) \sigma_{12}^{(1)} = -2\eta_0 \lambda_2 s(t)^2, \tag{S6a}$$

$$N_2^{(2)} + \lambda_1 \frac{dN_2^{(2)}}{dt} - (-\lambda_1 + \mu_1) s(t) \sigma_{12}^{(1)} + \frac{\alpha_1}{\eta_0} (\sigma_{12}^{(1)})^2 = \eta_0(\lambda_2 - \mu_2) s(t)^2. \tag{S6b}$$

Taking the Fourier transform of these equations gives the expressions:

$$\hat{N}_1^{(2)}(\omega) = \frac{1}{1 + i\lambda_1\omega} [2\lambda_1 \hat{s}(\omega) * \hat{\sigma}_{12}^{(1)}(\omega) - 2\eta_0 \lambda_2 \hat{s}(\omega) * \hat{s}(\omega)], \tag{S7a}$$

$$\hat{N}_2^{(2)}(\omega) = \frac{1}{1+i\lambda_1\omega}[(\mu_1-\lambda_1)\hat{s}(\omega)*\hat{\sigma}_{12}^{(1)}(\omega)+\eta_0(\lambda_2-\mu_2)\hat{s}(\omega)*\hat{s}(\omega)-\frac{\alpha_1}{\eta_0}\hat{\sigma}_{12}^{(1)}(\omega)*\hat{\sigma}_{12}^{(1)}(\omega)]. \quad \text{(S7b)}$$

Now, substituting into these equations the expression for $\hat{\sigma}_{12}^{(1)}(\omega)$ and making use of the convolution identity:

$$a(\omega)(b(\omega)*c(\omega)) = \frac{1}{2}\iint_{-\infty}^{\infty} a(\omega_1+\omega_2)[b(\omega_1)c(\omega_2)+b(\omega_2)c(\omega_1)]\delta(\omega-\omega_1-\omega_2)d\omega_1 d\omega_2, \quad \text{(S8)}$$

we recognize that:

$$\Psi_1^*(\omega_1,\omega_2) = \eta_0 \sum_{n=1}^{3} B_n \psi_n(\omega_1,\omega_2), \quad \text{(S9)}$$

$$\Psi_2^*(\omega_1,\omega_2) = \eta_0 \sum_{n=1}^{3} C_n \psi_n(\omega_1,\omega_2), \quad \text{(S10)}$$

with:

$$\psi_1(\omega_1,\omega_2) = \left( \frac{1}{1+i\lambda_1 \sum\limits_{j=1}^{2}\omega_j} \right), \quad \text{(S11a)}$$

$$\psi_2(\omega_1,\omega_2) = \frac{1}{2}\left( \frac{1}{1+i\lambda_1 \sum\limits_{j=1}^{2}\omega_j} \right) \left[ \sum_{j=1}^{2} \left( \frac{1+i\lambda_2\omega_j}{1+i\lambda_1\omega_j}, \right) \right], \quad \text{(S11b)}$$

$$\psi_3(\omega_1,\omega_2) = \left( \frac{1}{1+i\lambda_1 \sum\limits_{j=1}^{2}\omega_j} \right) \left[ \prod_{j=1}^{2} \left( \frac{1+i\lambda_2\omega_j}{1+i\lambda_1\omega_j} \right) \right], \quad \text{(S11c)}$$

and:

$$B_1 = -2\lambda_2, \quad B_2 = 2\lambda_1, \quad B_3 = 0, \quad \text{(S12)}$$

$$C_1 = \lambda_2 - \mu_2, \quad C_2 = -(\lambda_1 - \mu_1), \quad C_3 = -\alpha_1. \quad \text{(S13)}$$

## S1.2 Third Order Shear Stress

At third order in $\gamma_0$, we find that the third order contributions to the normal stresses are zero, and that the third order contribution to the shear stress is:

$$\sigma_{12}^{(3)} + \lambda_1 \frac{d\sigma_{12}^{(3)}}{dt} + \frac{1}{2}\lambda_1 s(t)(\sigma_{11}^{(2)} - \sigma_{22}^{(2)}) + \frac{1}{2}\mu_0 s(t)(\sigma_{11}^{(2)} + \sigma_{22}^{(2)} + \sigma_{33}^{(2)}) - \frac{1}{2}\mu_1 s(t)(\sigma_{11}^{(2)} + \sigma_{22}^{(2)})$$
$$- \frac{\alpha_0}{\eta_0}\sigma_{12}^{(1)}(\sigma_{11}^{(2)} + \sigma_{22}^{(2)} + \sigma_{33}^{(2)}) + \frac{\alpha_1}{\eta_0}\sigma_{12}^{(1)}(\sigma_{11}^{(2)} + \sigma_{22}^{(2)}) - \frac{2c_1\lambda_1}{\eta_0}s(t)(\sigma_{12}^{(1)})^2 - 2c_2\lambda_1 s(t)^2\sigma_{12}^{(1)}$$
$$- \frac{2c_3\lambda_1}{\eta_0^2}(\sigma_{12}^{(1)})^3 - \frac{2d_1\lambda_1}{\eta_0}s(t)(\sigma_{12}^{(1)})^2 - 2d_2\lambda_1 s(t)^2\sigma_{12}^{(1)} - \frac{2f_1\lambda_1}{\eta_0}s(t)(\sigma_{12}^{(1)})^2 - 2f_2\lambda_1 s(t)^2\sigma_{12}^{(1)}$$
$$- \frac{2f_3\lambda_1}{\eta_0^2}(\sigma_{12}^{(1)})^3 = 2\eta_0 d_3\lambda_1 s(t)^3 + 2\eta_0 f_4\lambda_1 s(t)^3. \quad \text{(S14)}$$

It is convenient here to define the trace of the stress tensor $T = \sigma_{11} + \sigma_{22} + \sigma_{33}$, and to note its second order response:

$$\hat{T}^{(2)}(\omega) = \frac{1}{1 + 3\zeta + i\lambda_1\omega}[\eta_0(3\nu_2 - 2\mu_2)\hat{s}(\omega) * \hat{s}(\omega) + (2\mu_1 - 3\nu_1)\hat{s}(\omega) * \hat{\sigma}_{12}^{(1)}(\omega)$$
$$+ \frac{1}{\eta_0}(3\beta_1 - 2\alpha_1)\hat{\sigma}_{12}^{(1)}(\omega) * \hat{\sigma}_{12}^{(1)}(\omega)], \quad \text{(S15)}$$

and to similarly note the second order response of the sum of the first and second normal stresses:

$$\hat{\sigma}_{11}^{(2)}(\omega) + \hat{\sigma}_{22}^{(2)}(\omega) = \frac{1}{1 + i\lambda_1\omega}[2(\mu_1 - \nu_1)\hat{s}(\omega) * \hat{\sigma}_{12}^{(1)}(\omega) + 2\eta_0(\nu_2 - \mu_2)\hat{s}(\omega) * \hat{s}(\omega)$$
$$+ \frac{2}{\eta_0}(\beta_1 - \alpha_1)\hat{\sigma}_{12}^{(1)}(\omega) * \hat{\sigma}_{12}^{(1)}(\omega) - 2\zeta\hat{T}^{(2)}(\omega)]. \quad \text{(S16)}$$

Using the trace and the previously defined normal stress differences, we may write the Fourier transform of the third order shear stress as:

$$\hat{\sigma}_{12}^{(3)}(\omega) = \frac{1}{1+i\lambda_1\omega}\Bigg[-\frac{1}{2}\lambda_1\hat{s}(\omega)*\hat{N}_1^{(2)}(\omega) - \frac{1}{2}\mu_0\hat{s}(\omega)*\hat{T}^{(2)}(\omega) + \frac{1}{2}\mu_1\hat{s}(\omega)*\Big(\hat{\sigma}_{11}^{(2)}(\omega) + \hat{\sigma}_{22}^{(2)}(\omega)\Big) + \frac{\alpha_0}{\eta_0}\hat{\sigma}_{12}^{(1)}(\omega)*\hat{T}^{(2)}(\omega) - \frac{\alpha_1}{\eta_0}\hat{\sigma}_{12}^{(1)}(\omega)*\Big(\hat{\sigma}_{11}^{(2)}(\omega)+\hat{\sigma}_{22}^{(2)}(\omega)\Big) + \frac{2\lambda_1}{\eta_0}(c_1+d_1+f_1)\hat{s}(\omega)*\hat{\sigma}_{12}^{(1)}(\omega)*\hat{\sigma}_{12}^{(1)}(\omega) + 2\lambda_1(c_2+d_2+f_2)\hat{s}(\omega)*\hat{s}(\omega)*\hat{\sigma}_{12}^{(1)}(\omega) + \frac{2\lambda_1}{\eta_0^2}(c_3+f_3)\hat{\sigma}_{12}^{(1)}(\omega)*\hat{\sigma}_{12}^{(1)}(\omega)*\hat{\sigma}_{12}^{(1)}(\omega) + 2\eta_0\lambda_1(d_3+f_4)\hat{s}(\omega)*\hat{s}(\omega)*\hat{s}(\omega)\Bigg]. \quad \text{(S17)}$$

Next, we substitute in the expressions for $\hat{N}_1^{(2)}(\omega)$, $\hat{T}^{(2)}(\omega)$, and $\hat{\sigma}_{33}^{(2)}(\omega)$, and apply the convolution identity:

$$a(\omega)\Big\{b(\omega)*\Big[c(\omega)\Big(d(\omega)*e(\omega)\Big)\Big]\Big\} \quad \text{(S18)}$$
$$= \frac{1}{6}\iiint_{-\infty}^{\infty} a(\omega_1+\omega_2+\omega_3)\Big[b(\omega_1)c(\omega_2+\omega_3)\Big(d(\omega_2)e(\omega_3)+d(\omega_3)e(\omega_2)\Big)$$
$$b(\omega_2)c(\omega_1+\omega_3)\Big(d(\omega_1)e(\omega_3)+d(\omega_3)e(\omega_1)\Big) + b(\omega_3)c(\omega_1+\omega_1)\Big(d(\omega_1)e(\omega_2)+d(\omega_2)e(\omega_1)\Big)\Big]$$
$$\times\,\delta(\omega-\omega_1-\omega_2-\omega_3)d\omega_1 d\omega_2 d\omega_3.$$

From this point, obtaining the solution for the third order complex viscosity is mostly an exercise in bookkeeping. Each of the basis functions in equation 20 from the main text arise via the convolution identity above applied to a different grouping of functions $a(\omega)$ through $e(\omega)$. The coefficients listed in Table 2 in the main text arise by the groupings of parameters associated with each different triple-convolution. For example, the following term arises in the fully expanded expression for $\hat{\sigma}_{12}^{(3)}$:

$$\Big(-\lambda_1^2+\mu_1(\mu_1-\nu_1)\Big)\left[\hat{s}(\omega)*\left(\frac{1}{1+i\lambda_1\omega}\hat{s}(\omega)*\hat{\sigma}_{12}^{(1)}(\omega)\right)\right]. \quad \text{(S19)}$$

The first expression in parenthesis is the coefficient $a_2^{(0)}$, and the triple convolution applied to the convolution identity gives the basis function $\Omega_2(\omega_1, \omega_2, \omega_2; 0, 0)$. The full expression for $\hat{\sigma}_{12}^{(3)}$ with all triple convolutions and coefficients is too unwieldy to write here; however, the remaining coefficients and basis functions can be found in an analogous manner to the above example.

# S2 Memory Kernel Relationships

In simple shear deformation, the deformation gradient tensor is:

$$\mathbf{F}(t,t') = \mathbf{I} + \gamma(t,t')\mathbf{e}_1\mathbf{e}_2, \tag{S20}$$

so the relative finite strain tensor is:

$$\boldsymbol{\gamma}(t,t') = \gamma^2(t,t')\mathbf{e}_1\mathbf{e}_1 + \gamma(t,t')(\mathbf{e}_1\mathbf{e}_2 + \mathbf{e}_2\mathbf{e}_1). \tag{S21}$$

The components of the stress tensor are therefore given by:

$$\begin{aligned}\sigma_{12}(t) = &\int_{-\infty}^{t} M_I(t-t')\gamma(t,t')dt' \\ &+ \iiint_{-\infty}^{t} \left[M_{II}(t-t',t-t'')\left(\delta(t'''-t') + \delta(t'''-t'')\right) + 2M_{III}(t-t',t-t'',t-t''')\right. \\ &\left. +2M_{IV}(t-t',t-t'',t-t''')\right]\gamma(t,t')\gamma(t,t'')\gamma(t,t''')dt'dt''dt''' + O(\gamma^5),\end{aligned} \tag{S22}$$

$$\sigma_{11}(t) = \iint_{-\infty}^{t} \left[M_I(t-t')\delta(t''-t') + 2M_{II}(t-t',t-t'')\right]\gamma(t,t')\gamma(t,t'')dt'dt'' + O(\gamma^4), \tag{S23}$$

$$\sigma_{22}(t) = \iint_{-\infty}^{t} 2M_{II}(t-t',t-t'')\gamma(t,t')\gamma(t,t'')dt'dt'' + O(\gamma^4). \tag{S24}$$

The normal stress differences are therefore:

$$\sigma_{11}(t) - \sigma_{22}(t) = \iint_{-\infty}^{t} M_I(t-t')\delta(t''-t')\gamma(t,t')\gamma(t,t'')dt'dt'' + O(\gamma^4), \tag{S25}$$

$$\sigma_{22}(t) - \sigma_{33}(t) = \iint_{-\infty}^{t} 2M_{II}(t-t', t-t'')\gamma(t,t')\gamma(t,t'')dt'dt'' + O(\gamma^4). \tag{S26}$$

The expansions can be represented in frequency space instead. To do so, we make the change of variables $s_1 = t - t'$, $s_2 = t - t''$, and $s_3 = t - t'''$. The strain protocol can be represented in terms of its Fourier transform:

$$\gamma(t,t') = \gamma(t) - \gamma(t-s) = \int_{-\infty}^{\infty} e^{i\omega t}\left(1 - e^{-i\omega s}\right)\hat{\gamma}(\omega)d\omega. \tag{S27}$$

At first order, we find that:

$$\begin{aligned}
\sigma_{12}^{(1)}(t) &= \int_{-\infty}^{\infty} e^{i\omega_1 t}\hat{\gamma}(\omega_1)d\omega_1 \int_0^{\infty} M_I(s_1)(1 - e^{-i\omega_1 s_1})ds_1 \\
&= \int_{-\infty}^{\infty} e^{i\omega_1 t}\hat{\gamma}(\omega_1)d\omega_1 \int_0^{\infty}\int_{-\infty}^{\infty} M_I^*(\omega)e^{i\omega s_1}(1 - e^{-i\omega_1 s_1})d\omega ds_1 \\
&= \int_{-\infty}^{\infty} e^{i\omega_1 t}\hat{\gamma}(\omega_1)d\omega_1 \int_0^{\infty}\int_{-\infty}^{\infty} M_I^*(\omega)e^{i\omega s_1}(1 - e^{-i\omega_1 s_1)})d\omega ds_1 \\
&= \left[M_I^*(0) - M_I^*(\omega)\right]\hat{\gamma}(\omega)
\end{aligned} \tag{S28}$$

where:

$$M_I^*(\omega) = \int_0^{\infty} e^{-i\omega s} M_I(\sigma)ds. \tag{S29}$$

Therefore, we see that $G^*(\omega) = [M_I^*(0) - M_I^*(\omega)]$. At second order:

$$\begin{aligned}
\sigma_{11}^{(2)}(t) - \sigma_{22}^{(2)}(t) = &\iint_{-\infty}^{\infty} e^{i(\omega_1+\omega_2)t}\hat{\gamma}(\omega_1)\hat{\gamma}(\omega_2)d\omega_1 d\omega_2 \\
&\times \iint_0^{\infty} M_I(s_1)\delta(s_1 - s_2)(1 - e^{-i\omega_1 s_1})(1 - e^{-i\omega_2 s_2})ds_1 ds_2.
\end{aligned} \tag{S30}$$

Therefore, the first normal stress difference is:

$$\hat{\sigma}_{11}^{(2)}(\omega) - \hat{\sigma}_{22}^{(2)}(\omega) = \iint_{-\infty}^{\infty} \Psi_1^*(\omega_1, \omega_2)\hat{\gamma}(\omega_1)\hat{\gamma}(\omega_2)\delta(\omega - \omega_1 - \omega_2)d\omega_1 d\omega_2, \tag{S31}$$

with:

$$\begin{aligned}\Psi_1^*(\omega_1, \omega_2) &= \iint_0^{\infty} M_I(s_1)\delta(s_1 - s_2)(1 - e^{-i\omega_1 s_1})(1 - e^{-i\omega_2 s_2})ds_1 ds_2 \\ &= M_I^*(0) - M_I^*(\omega_1) - M_I^*(\omega_2) + M_I^*(\omega_1 + \omega_2) \\ &= G^*(\omega_1) + G^*(\omega_2) - G^*(\omega_1 + \omega_2).\end{aligned} \tag{S32}$$

The second normal stress difference is:

$$\hat{\sigma}_{22}^{(2)}(\omega) - \hat{\sigma}_{33}^{(2)}(\omega) = \iint_{-\infty}^{\infty} \Psi_2^*(\omega_1, \omega_2)\hat{\gamma}(\omega_1)\hat{\gamma}(\omega_2)\delta(\omega - \omega_1 - \omega_2)d\omega_1 d\omega_2 \tag{S33}$$

with:

$$\begin{aligned}\Psi_2^*(\omega_1, \omega_2) &= \iint_0^{\infty} 2M_{II}(s_1, s_2)(1 - e^{-i\omega_1 s_1})(1 - e^{-i\omega_2 s_2})ds_1 ds_2 \\ &= 2\left[M_{II}^*(0,0) - \sum_{j=1}^{2} M_{II}^*(\omega_j, 0) + M_{II}^*(\omega_1, \omega_2)\right],\end{aligned} \tag{S34}$$

where:

$$M_{II}^*(\omega_1, \omega_2) = \iint_0^{\infty} e^{-i\omega_1 s_2 - i\omega_2 s_2} M_{II}(s_1, s_2)ds_1 ds_2. \tag{S35}$$

At third order, the shear stress is:

$$\hat{\sigma}_{12}^{(3)}(\omega) = \iiint_{-\infty}^{\infty} G_3^*(\omega_1, \omega_2, \omega_3)\hat{\gamma}(\omega_1)\hat{\gamma}(\omega_2)\hat{\gamma}(\omega_3)\delta(\omega - \sum_j \omega_j)d\omega_1 d\omega_2 d\omega_3, \tag{S36}$$

where the third order complex modulus is:

$$
\begin{aligned}
G_3^*(\omega_1, \omega_2, \omega_3) = & \iiint_0^\infty \left[M_{II}(s_1, s_2)\left(\delta(s_1 - s_3) + \delta(s_2 - s_3)\right) + 2M_{III}(s_1, s_2, s_3)\right. \\
& \left. +2M_{IV}(s_1, s_2, s_3)\right](1 - e^{-i\omega_1 s_1})(1 - e^{-i\omega_2 s_2})(1 - e^{-i\omega_3 s_3})ds_1 ds_2 ds_3 \\
= & \, 2\left[M_{II}^*(0,0) - M_{II}^*(\omega_1, 0) - M_{II}^*(0, \omega_2) + M_{II}^*(\omega_1, \omega_2)\right] \\
& - M_{II}^*(\omega_3, 0) - M_{II}^*(0, \omega_3) + M_{II}^*(\omega_1 + \omega_3, 0) + M_{II}^*(\omega_1, \omega_3) \\
& + M_{II}^*(0, \omega_2 + \omega_3) + M_{II}^*(\omega_3, \omega_2) - M_{II}^*(\omega_1 + \omega_3, \omega_2) - M_{II}^*(\omega_1, \omega_2 + \omega_3) \\
& + 2\left[M_{III}^*(0,0,0) - \sum_j M_{III}^*(\omega_j, 0, 0) + \frac{1}{2}\sum_{j=1}^{3}\sum_{k \neq j} M_{III}^*(\omega_j, \omega_k) - M_{III}^*(\omega_1, \omega_2, \omega_3)\right] \\
& + 2\left[M_{IV}^*(0,0,0) - \sum_j M_{IV}^*(\omega_j, 0, 0) + \frac{1}{2}\sum_{j=1}^{3}\sum_{k \neq j} M_{IV}^*(\omega_j, \omega_k) - M_{IV}^*(\omega_1, \omega_2, \omega_3)\right].
\end{aligned}
\tag{S37}
$$

This expression is not permutation-symmetric due to the asymmetric contributions from $M_{II}^*$. After symmetrizing, it becomes:

$$
\begin{aligned}
G_3^*(\omega_1, \omega_2, \omega_3) = & \frac{1}{3}\{4\left[M_{II}^*(0,0) - M_{II}^*(\omega_1, 0) - M_{II}^*(0, \omega_2) + M_{II}^*(\omega_1, \omega_2)\right] \\
& + 4\left[M_{II}^*(0,0) - M_{II}^*(\omega_1, 0) - M_{II}^*(0, \omega_3) + M_{II}^*(\omega_1, \omega_3)\right] \\
& + 4\left[M_{II}^*(0,0) - M_{II}^*(\omega_3, 0) - M_{II}^*(0, \omega_2) + M_{II}^*(\omega_3, \omega_2)\right] \\
& - 2\left[M_{II}^*(0,0) - M_{II}^*(\omega_1 + \omega_3, 0) - M_{II}^*(0, \omega_2) + M_{II}^*(\omega_1 + \omega_3, \omega_2)\right] \\
& - 2\left[M_{II}^*(0,0) - M_{II}^*(\omega_1 + \omega_2, 0) - M_{II}^*(0, \omega_3) + M_{II}^*(\omega_1 + \omega_2, \omega_3)\right] \\
& - 2\left[M_{II}^*(0,0) - M_{II}^*(\omega_2 + \omega_3, 0) - M_{II}^*(0, \omega_1) + M_{II}^*(\omega_2 + \omega_3, \omega_1)\right] \\
& + 2\left[M_{III}^*(0,0,0) - \sum_j M_{III}^*(\omega_j, 0, 0) + \frac{1}{2}\sum_{j=1}^{3}\sum_{k \neq j} M_{III}^*(\omega_j, \omega_k) - M_{III}^*(\omega_1, \omega_2, \omega_3)\right] \\
& + 2\left[M_{IV}^*(0,0,0) - \sum_j M_{IV}^*(\omega_j, 0, 0) + \frac{1}{2}\sum_{j=1}^{3}\sum_{k \neq j} M_{IV}^*(\omega_j, \omega_k) - M_{IV}^*(\omega_1, \omega_2, \omega_3)\right].
\end{aligned}
\tag{S38}
$$

The dependence of $M_{II}^*$ can be expressed in terms of $\Psi_2^*$ instead, giving:

$$G_3^*(\omega_1,\omega_2,\omega_3) = \frac{1}{3}\sum_{j=1}^{3}\sum_{k\neq j}\Psi_2^*(\omega_j,\omega_k) - \frac{1}{3}\sum_{j=1}^{3}\Psi_2^*(\omega_j,\sum_{k\neq j}\omega_k) \quad \text{(S39)}$$

$$+ K_{III}^*(\omega_1,\omega_2,\omega_3) + K_{IV}^*(\omega_1,\omega_2,\omega_3), \quad \text{(S40)}$$

with:

$$K_{III}^*(\omega_1,\omega_2,\omega_3) = 2\Bigg[M_{III}^*(0,0,0) - \sum_j M_{III}^*(\omega_j,0,0) \quad \text{(S41)}$$
$$+ \frac{1}{2}\sum_{j=1}^{3}\sum_{k\neq j} M_{III}^*(\omega_j,\omega_k) - M_{III}^*(\omega_1,\omega_2,\omega_3)\Bigg],$$

$$K_{IV}^*(\omega_1,\omega_2,\omega_3) = 2\Bigg[M_{IV}^*(0,0,0) - \sum_j M_{IV}^*(\omega_j,0,0) \quad \text{(S42)}$$
$$+ \frac{1}{2}\sum_{j=1}^{3}\sum_{k\neq j} M_{IV}^*(\omega_j,\omega_k) - M_{IV}^*(\omega_1,\omega_2,\omega_3)\Bigg].$$

# S3 Shear Startup Basis Functions

The shear startup basis functions $\Sigma_n(t)$ are obtained by taking the three-dimensional inverse Fourier transform of the basis functions $\Omega_n(\omega_1,\omega_2,\omega_3)$:

$$\mathcal{F}^{-1}_{\omega_1,\omega_2,\omega_3}[\Omega_n(\omega_1,\omega_2,\omega_3)] = \frac{1}{(2\pi)^3}\iiint_{-\infty}^{\infty}\Omega_n(\omega_1,\omega_2,\omega_3)e^{i(\omega_1\tau_1+\omega_2\tau_2+\omega_3\tau_3)}d\omega_1 d\omega_2 d\omega_3 \quad \text{(S43)}$$

and then taking the following integral:

$$\Sigma_n(t) = \iiint_{-\infty}^{t}\mathcal{F}^{-1}_{\omega_1,\omega_2,\omega_3}[\Omega_n(\omega_1,\omega_2,\omega_3)](\tau_1,\tau_2,\tau_3)d\tau_1 d\tau_2 d\tau_3. \quad \text{(S44)}$$

With the non-dimensionalization $\tau = t/\lambda_1$ and $\breve{\lambda}_2 = \lambda_2/\lambda_1$ (also commonly denoted as $\beta$), the resulting time-domain basis functions are:

$$\Sigma_1(t) = 1 - e^{-\tau} - \tau e^{-\tau}, \tag{S45a}$$

$$\Sigma_2(t) = 1 - e^{-\tau} - \tau e^{-\tau} - \frac{1}{2}\left(1 - \breve{\lambda}_2\right)\tau^2 e^{-\tau}, \tag{S45b}$$

$$\Sigma_3(t) = 1 - e^{-\tau} - \tau e^{-\tau} + \left(1 - \breve{\lambda}_2\right)\left(e^{-\tau} - e^{-2\tau} - \tau e^{-\tau}\right), \tag{S45c}$$

$$\begin{aligned}\Sigma_4(t) = &1 - e^{-\tau} - \tau e^{-\tau} - \frac{1}{2}\left(1 - \breve{\lambda}_2\right)\tau^2 e^{-\tau} + \left(1 - \breve{\lambda}_2\right)\left(e^{-\tau} - \tau e^{-\tau} - e^{-2\tau}\right) \\ &+ \left(1 - \breve{\lambda}_2\right)^2\left(e^{-\tau} - e^{-2\tau} - \tau e^{-2\tau}\right),\end{aligned} \tag{S45d}$$

$$\Sigma_5(t) = 1 - e^{-\tau} - \tau e^{-\tau} - \left(1 - \breve{\lambda}_2\right)\tau^2 e^{-\tau} - \left(1 - \breve{\lambda}_2\right)^2\left(e^{-\tau} - \tau e^{-\tau} - e^{-2\tau}\right), \tag{S45e}$$

$$\begin{aligned}\Sigma_6(t) = &1 - e^{-\tau} - \tau e^{-\tau} - \left(1 - \breve{\lambda}_2\right)\tau^2 e^{-\tau} + \left(1 - \breve{\lambda}_2\right)\left(e^{-\tau} - \tau e^{-\tau} - e^{-2\tau}\right) \\ &+ \left(1 - \breve{\lambda}_2\right)^2\left(e^{-\tau} + \tau e^{-\tau} - e^{-2\tau} - 2\tau e^{-2\tau}\right) - \frac{1}{2}\left(1 - \breve{\lambda}_2\right)^3\left(e^{-\tau} - 2e^{-2\tau} + e^{-3\tau}\right).\end{aligned} \tag{S45f}$$

# S4 Derivation of the Startup Viscosity for the Oldroyd 8-Constant Model

When subjected to the startup of steady shear flow ($\mathbf{u} = \dot{\gamma}_0 H(t) x_2 \mathbf{e}_1$, where $H(t)$ represents the Heaviside step function), the Oldroyd-8 constant model can be written:

$$\begin{aligned}\frac{d\breve{\sigma}_{12}(\tau)}{d\tau} = &-\breve{\sigma}_{12}(\tau) - \frac{1}{2}\mathrm{Wi}(1 + \breve{\mu}_0 - \breve{\mu}_1)\breve{N}_1(\tau)H(\tau) - \mathrm{Wi}(\breve{\mu}_0 - \breve{\mu}_1)\breve{N}_2(\tau)H(\tau) \\ &- \mathrm{Wi}\left(\frac{3}{2}\breve{\mu}_0 - \breve{\mu}_1\right)\breve{\sigma}_{33}(\tau)H(\tau) + \mathrm{Wi}H(\tau) + \mathrm{Wi}\,\breve{\lambda}_2\delta(\tau)\end{aligned} \tag{S46a}$$

$$\frac{d\breve{N}_1(\tau)}{d\tau} = -\breve{N}_1(\tau) + 2\text{Wi}\,\breve{\sigma}_{12}(\tau)H(\tau) - 2\text{Wi}^2\breve{\lambda}_2 H(\tau) \tag{S46b}$$

$$\frac{d\breve{N}_2(\tau)}{d\tau} = -\breve{N}_2(\tau) - \text{Wi}(1-\breve{\mu}_1)\breve{\sigma}_{12}(\tau)H(\tau) + \text{Wi}^2(\breve{\lambda}_2 - \breve{\mu}_2)H(\tau) \tag{S46c}$$

$$\frac{d\breve{\sigma}_{33}(\tau)}{d\tau} = -\breve{\sigma}_{33}(\tau) - \text{Wi}\,\breve{\nu}_1\breve{\sigma}_{12}(\tau)H(\tau) + \text{Wi}^2\breve{\nu}_2 H(\tau). \tag{S46d}$$

Here, we adopt the notation of Saengow et. al [1], with $\breve{\mu}_i = \mu_i/\lambda_1$, $\breve{\lambda}_2 = \lambda_2/\lambda_1$, $\breve{\nu}_i = \nu_i/\lambda_1$, $\breve{\sigma}_{12} = \sigma_{12}/(\eta_0/\lambda_1)$, $\breve{N}_1 = (\sigma_{11} - \sigma_{22})/(\eta_0/\lambda_1)$, $\breve{N}_2 = (\sigma_{22} - \sigma_{33})/(\eta_0/\lambda_1)$, $\breve{\sigma}_{33} = \sigma_{33}/(\eta_0/\lambda_1)$, $\tau = t/\lambda_1$, and $\text{Wi} = \dot{\gamma}_0\lambda_1$.

Taking the Laplace transforms of these equations gives (with $\hat{f}$ representing the Laplace transform of a normalized function $\breve{f}(\tau)$, and $s$ representing the conjugate variable to $\tau$):

$$s\hat{\sigma}_{12} = -\hat{\sigma}_{12} - \frac{1}{2}(1+\breve{\mu}_0 - \breve{\mu}_1)\hat{N}_1\text{Wi} - (\breve{\mu}_0 - \breve{\mu}_1)\hat{N}_2\text{Wi} - \left(\frac{3}{2}\breve{\mu}_0 - \breve{\mu}_1\right)\hat{\sigma}_{33}\text{Wi} + \frac{\text{Wi}}{s} + \breve{\lambda}_2\text{Wi} \tag{S47a}$$

$$s\hat{N}_1 = -\hat{N}_1 + 2\hat{\sigma}_{12}\text{Wi} - \frac{2\breve{\lambda}_2\text{Wi}^2}{s} \tag{S47b}$$

$$s\hat{N}_2 = -\hat{N}_2 - (1-\breve{\mu}_1)\hat{\sigma}_{12}\text{Wi} + \frac{(\breve{\lambda}_2 - \breve{\mu}_2)\text{Wi}^2}{s} \tag{S47c}$$

$$s\hat{\sigma}_{33} = -\hat{\sigma}_{33} - \breve{\nu}_1\hat{\sigma}_{12}\text{Wi} + \frac{\breve{\nu}_2\text{Wi}^2}{s}. \tag{S47d}$$

Solving for the normal stress functions and substituting into the equation for the shear stress, then lumping constants according to the two lumped constants:

$$\breve{A}_1 = \frac{1}{\lambda_1}A_1 = \breve{\lambda}_2 - \breve{\mu}_1(\breve{\mu}_2 - \breve{\nu}_2) + \breve{\mu}_0\left(\breve{\mu}_2 - \frac{3}{2}\breve{\nu}_2\right), \tag{S48a}$$

$$\breve{A}_2 = \frac{1}{\lambda_1}A_2 = -1 + \breve{\mu}_1(\breve{\mu}_1 - \breve{\nu}_1) - \breve{\mu}_0\left(\breve{\mu}_1 - \frac{3}{2}\breve{\nu}_1\right), \tag{S48b}$$

we find that

$$\hat{\sigma}_{12}\left[(s+1)^2 - \breve{A}_2\mathrm{Wi}^2\right] = \frac{\breve{A}_1\mathrm{Wi}^3}{s} + \frac{\mathrm{Wi}(1+s)}{s} + \breve{\lambda}_2\mathrm{Wi}(1+s). \tag{S49}$$

The Laplace transform can now be inverted by noting that

$$\mathcal{L}^{-1}\left[\frac{\hat{f}(s)}{s}\right](\tau) = \int_0^\tau f(t)dt, \tag{S50}$$

$$\mathcal{L}^{-1}\left[\frac{b}{(s-a)^2+b^2}\right](\tau) = e^{a\tau}\sin b\tau, \tag{S51}$$

$$\mathcal{L}^{-1}\left[\frac{s-a}{(s-a)^2+b^2}\right](\tau) = e^{a\tau}\cos b\tau, \tag{S52}$$

$$\int_0^\tau e^{-t}\sin bt = \frac{e^{-\tau}}{1+b^2}\left[-\sin b\tau - b\cos b\tau\right] + \frac{b}{1+b^2}, \tag{S53}$$

and

$$\int_0^\tau e^{-t}\cos bt = \frac{e^{-\tau}}{1+b^2}\left[-\cos b\tau + b\sin b\tau\right] + \frac{1}{1+b^2}. \tag{S54}$$

Applying these identities and simplifying, we find that

$$\begin{aligned}\breve{\sigma}_{12}(\tau) = -\mathrm{Wi}\,e^{-\tau}&\left[\left(\frac{1+\breve{A}_1\mathrm{Wi}^2}{1-\breve{A}_2\mathrm{Wi}^2} - \breve{\lambda}_2\right)\cos\left(\sqrt{-\breve{A}_2}\mathrm{Wi}\tau\right)\right.\\ &\left.+\frac{1}{\sqrt{-\breve{A}_2}}\frac{\breve{A}_1+\breve{A}_2}{1-\breve{A}_2\mathrm{Wi}^2}\mathrm{Wi}\sin\left(\sqrt{-\breve{A}_2}\mathrm{Wi}\tau\right)\right] + \mathrm{Wi}\frac{1+\breve{A}_1\mathrm{Wi}^2}{1-\breve{A}_2\mathrm{Wi}^2}.\end{aligned} \tag{S55}$$

Now, defining $\breve{\eta}^+(\tau, \mathrm{Wi}) \equiv \breve{\sigma}_{12}/\mathrm{Wi}$, we find that

$$\begin{aligned}\breve{\eta}^+(\tau, \mathrm{Wi}) = -e^{-\tau}&\left[\left(\frac{1+\breve{A}_1\mathrm{Wi}^2}{1-\breve{A}_2\mathrm{Wi}^2} - \breve{\lambda}_2\right)\cos\left(\sqrt{-\breve{A}_2}\mathrm{Wi}\tau\right)\right.\\ &\left.+\frac{1}{\sqrt{-\breve{A}_2}}\frac{\breve{A}_1+\breve{A}_2}{1-\breve{A}_2\mathrm{Wi}^2}\mathrm{Wi}\sin\left(\sqrt{-\breve{A}_2}\mathrm{Wi}\tau\right)\right] + \frac{1+\breve{A}_1\mathrm{Wi}^2}{1-\breve{A}_2\mathrm{Wi}^2}.\end{aligned} \tag{S56}$$

where $\tau = t/\lambda_1$.

This solution differs slightly from that of Saengow et. al. [1], which can be seen most clearly by realizing that $\breve{A}_2 = -\breve{\sigma}_1$ and $\breve{A}_1 = \breve{\sigma}_2$, where $\breve{\sigma}_1$ and $\breve{\sigma}_2$ are the lumped constants defined by Saengow. In particular, the expression in [1] omits the retardation term $-\breve{\lambda}_2$ in the first parenthesis within the square brackets. This corresponds to the instantaneous jump in the viscous solvent stress upon the inception of steady shear flow. However, the solution presented here is consistent with the asymptotic expansion in terms of the basis functions $\Sigma_n(t)$, and consistent with the solution noted by other authors for the corotational Jeffreys model [2].

# References


[1] C. Saengow, A. J. Giacomin, N. Grizzuti, and R. Pasquino, “Startup steady shear flow from the Oldroyd 8-constant framework,” *Physics of Fluids*, vol. 31, no. 6, 063101, 2019.

[2] R. B. Bird, R. C. Armstrong, and O. Hassager, *Dynamics of Polymeric Liquids, Volume 1: Fluid Mechanics.* John Wiley & Sons, Inc., 2 ed., 1987.
